# Supplementary material for: Cross-lingual Calibration of Pre-Generation Success Probes for Multilingual LLM Routing
Source: arXiv:2610.06216 source file (2026-10-05)
Supplement: Supplementary file 1 [file appendix_all_source_auroc.tex]

\begin{table*}[t]
\centering
\scriptsize
\setlength{\tabcolsep}{3pt}
\begin{tabular}{lrrrrrrrrrr}
\toprule
Source $\backslash$ target & Eng & Ara & Chi & Fre & Ita & Rus & Swa & Tel & Tha & Tur \\
\midrule
Eng & 0.74 & 0.71 & 0.72 & 0.71 & 0.69 & 0.71 & 0.67 & 0.70 & 0.70 & 0.68 \\
Ara & 0.68 & 0.75 & 0.70 & 0.70 & 0.70 & 0.72 & 0.72 & 0.71 & 0.71 & 0.69 \\
Chi & 0.67 & 0.69 & 0.73 & 0.68 & 0.66 & 0.69 & 0.69 & 0.67 & 0.70 & 0.64 \\
Fre & 0.69 & 0.71 & 0.70 & 0.74 & 0.72 & 0.73 & 0.68 & 0.67 & 0.70 & 0.68 \\
Ita & 0.70 & 0.72 & 0.69 & 0.72 & 0.73 & 0.73 & 0.70 & 0.69 & 0.71 & 0.68 \\
Rus & 0.70 & 0.72 & 0.73 & 0.71 & 0.70 & 0.75 & 0.72 & 0.71 & 0.71 & 0.69 \\
Swa & 0.65 & 0.68 & 0.66 & 0.66 & 0.66 & 0.68 & 0.77 & 0.71 & 0.69 & 0.67 \\
Tel & 0.67 & 0.71 & 0.68 & 0.67 & 0.68 & 0.69 & 0.73 & 0.77 & 0.71 & 0.69 \\
Tha & 0.66 & 0.70 & 0.67 & 0.67 & 0.65 & 0.69 & 0.72 & 0.72 & 0.74 & 0.70 \\
Tur & 0.68 & 0.71 & 0.70 & 0.69 & 0.69 & 0.69 & 0.72 & 0.71 & 0.71 & 0.73 \\
\bottomrule
\end{tabular}
\caption{All-source transfer at each model's shared reporting layer, averaged over
the eight models. Values are rollout AUROC. The diagonal is the same-language
oracle; off-diagonal cells are the 90 directed cross-language pairs.}
\label{tab:all-source}
\end{table*}
