# Supplementary material for: Cross-lingual Calibration of Pre-Generation Success Probes for Multilingual LLM Routing
Source: arXiv:2610.06216 source file (2026-10-05)
Supplement: Supplementary file 2 [file appendix_anchor_margin.tex]

\begin{table}[t]
\centering
\scriptsize
\resizebox{\columnwidth}{!}{%
\begin{tabular}{llrrrr}
\toprule
Predictor & Val. choice & $\lambda$ & Margin & Success & Saving \\
\midrule
english\_raw & anchor match & 0.000 & 0.030 & 84.5 & 8.3 \\
english\_model\_calibrated & anchor match & 0.050 & 0.050 & 84.5 & 4.5 \\
pooled\_raw & anchor match & 0.200 & 0.050 & 84.1 & 25.9 \\
\bottomrule
\end{tabular}%
}
\caption{Appendix anchor-margin policies selected on validation with the same
0.1-point anchor tolerance; ``no match'' means the fixed grid did not attain
it. These are not the main router, which uses the unmodified utility argmax.}
\label{tab:anchor-margin}
\end{table}
