# Supplementary material for: Cross-lingual Calibration of Pre-Generation Success Probes for Multilingual LLM Routing
Source: arXiv:2610.06216 source file (2026-10-05)
Supplement: Supplementary file 3 [file appendix_costs.tex]

\begin{table}[t]
\centering
\small
\resizebox{\columnwidth}{!}{%
\begin{tabular}{lrrrr}
\toprule
Model & Gen. (m\$) & Prefill (m\$) & ETD rel. & Prior rel. \\
\midrule
Qwen3-0.6B & 0.036 & 0.002 & 0.015 & 0.011 \\
Qwen3-1.7B & 0.401 & 0.006 & 0.124 & 0.120 \\
Qwen3-4B & 0.822 & 0.014 & 0.246 & 0.246 \\
Qwen3-8B & 1.237 & 0.027 & 0.375 & 0.371 \\
Qwen3.5-4B & 1.217 & 0.012 & 0.365 & 0.361 \\
Qwen3.5-9B & 2.285 & 0.028 & 0.683 & 0.679 \\
oss-low & 1.158 & 0.046 & 0.358 & 0.354 \\
oss-high & 3.359 & 0.046 & 1.004 & 1.000 \\
\bottomrule
\end{tabular}%
}
\caption{One-generation training-mean costs. ETD cost includes the shared encoder
prefill and the selected target prefill (reused when the encoder is selected);
prior cost needs no encoder. Relative costs use the standalone anchor as 1.}
\label{tab:costs}
\end{table}
