# Supplementary material for: Cross-lingual Calibration of Pre-Generation Success Probes for Multilingual LLM Routing
Source: arXiv:2610.06216 source file (2026-10-05)
Supplement: Supplementary file 4 [file appendix_majority_auroc.tex]

\begin{table}[t]
\centering
\small
\resizebox{\columnwidth}{!}{%
\begin{tabular}{llrr}
\toprule
Model & Training & Rollout AUROC & Majority AUROC \\
\midrule
Qwen3-0.6B & English & 0.710 & 0.751 \\
Qwen3-0.6B & Pooled & 0.718 & 0.766 \\
Qwen3-1.7B & English & 0.741 & 0.776 \\
Qwen3-1.7B & Pooled & 0.766 & 0.797 \\
Qwen3-4B & English & 0.729 & 0.749 \\
Qwen3-4B & Pooled & 0.741 & 0.760 \\
Qwen3-8B & English & 0.739 & 0.762 \\
Qwen3-8B & Pooled & 0.743 & 0.767 \\
Qwen3.5-4B & English & 0.684 & 0.716 \\
Qwen3.5-4B & Pooled & 0.737 & 0.770 \\
Qwen3.5-9B & English & 0.690 & 0.708 \\
Qwen3.5-9B & Pooled & 0.723 & 0.743 \\
oss-low & English & 0.681 & 0.699 \\
oss-low & Pooled & 0.695 & 0.711 \\
oss-high & English & 0.603 & 0.620 \\
oss-high & Pooled & 0.669 & 0.687 \\
\bottomrule
\end{tabular}%
}
\caption{Compatibility comparison between rollout-weighted AUROC and the legacy
majority-of-five target, at the frozen shared layer.}
\label{tab:majority}
\end{table}
