# Supplementary material for: Cross-lingual Calibration of Pre-Generation Success Probes for Multilingual LLM Routing
Source: arXiv:2610.06216 source file (2026-10-05)
Supplement: Supplementary file 5 [file appendix_model_mixes.tex]

\begin{table*}[t]
\centering
\scriptsize
\setlength{\tabcolsep}{3pt}
\begin{tabular}{lrrrrrrrr}
\toprule
Router & Qwen3-0.6B & Qwen3-1.7B & Qwen3-4B & Qwen3-8B & Qwen3.5-4B & Qwen3.5-9B & oss-low & oss-high \\
\midrule
language\_priors & 0.0 & 0.0 & 0.0 & 0.0 & 11.1 & 55.6 & 0.0 & 33.3 \\
pooled\_raw & 0.2 & 0.7 & 3.8 & 0.4 & 14.5 & 28.6 & 13.0 & 38.9 \\
\bottomrule
\end{tabular}
\caption{Selected-model percentages at validation-selected anchor-matching test
operating points.}
\label{tab:model-mixes}
\end{table*}
