# Supplementary material for: Cross-lingual Calibration of Pre-Generation Success Probes for Multilingual LLM Routing
Source: arXiv:2610.06216 source file (2026-10-05)
Supplement: Supplementary file 6 [file appendix_prediction_intervals.tex]

\begin{table*}[t]
\centering
\scriptsize
\setlength{\tabcolsep}{2.5pt}
\resizebox{\textwidth}{!}{%
\begin{tabular}{llrrrrrr}
\toprule
Model & Predictor & AUROC & Brier & NLL & ECE & Intercept & Slope \\
\midrule
\multirow{3}{*}{Qwen3-0.6B} & English & 0.710 [0.666,0.749] & 0.120 [0.110,0.131] & 0.624 [0.545,0.711] & 0.116 [0.109,0.124] & -1.311 [-1.631,-1.042] & 0.408 [0.283,0.566] \\
 & Pooled & 0.718 [0.671,0.759] & 0.099 [0.088,0.110] & 0.450 [0.392,0.514] & 0.038 [0.037,0.052] & -1.530 [-1.809,-1.142] & 0.158 [0.097,0.325] \\
 & Oracle & 0.769 [0.728,0.804] & 0.095 [0.085,0.105] & 0.395 [0.346,0.454] & 0.031 [0.029,0.044] & -1.120 [-1.518,-0.557] & 0.335 [0.204,0.613] \\
\addlinespace[1pt]
\multirow{3}{*}{Qwen3-1.7B} & English & 0.741 [0.707,0.771] & 0.190 [0.182,0.198] & 0.585 [0.560,0.611] & 0.129 [0.124,0.144] & -0.266 [-0.424,-0.117] & 1.381 [1.165,1.617] \\
 & Pooled & 0.766 [0.735,0.793] & 0.161 [0.152,0.171] & 0.554 [0.513,0.601] & 0.042 [0.045,0.063] & -0.317 [-0.490,-0.136] & 0.656 [0.499,0.867] \\
 & Oracle & 0.778 [0.749,0.803] & 0.157 [0.147,0.167] & 0.540 [0.499,0.585] & 0.037 [0.040,0.058] & -0.332 [-0.505,-0.105] & 0.585 [0.437,0.813] \\
\addlinespace[1pt]
\multirow{3}{*}{Qwen3-4B} & English & 0.729 [0.698,0.758] & 0.213 [0.205,0.220] & 0.624 [0.599,0.653] & 0.125 [0.115,0.146] & 0.301 [0.140,0.479] & 1.220 [0.927,1.554] \\
 & Pooled & 0.741 [0.713,0.768] & 0.190 [0.183,0.198] & 0.573 [0.548,0.600] & 0.043 [0.046,0.063] & 0.050 [-0.092,0.192] & 0.924 [0.750,1.160] \\
 & Oracle & 0.758 [0.729,0.783] & 0.183 [0.175,0.192] & 0.558 [0.534,0.584] & 0.031 [0.037,0.055] & 0.025 [-0.096,0.163] & 0.895 [0.754,1.078] \\
\addlinespace[1pt]
\multirow{3}{*}{Qwen3-8B} & English & 0.739 [0.709,0.767] & 0.212 [0.204,0.220] & 0.613 [0.594,0.631] & 0.118 [0.107,0.136] & 0.450 [0.334,0.570] & 1.386 [1.204,1.591] \\
 & Pooled & 0.743 [0.713,0.771] & 0.196 [0.187,0.205] & 0.580 [0.553,0.613] & 0.037 [0.042,0.062] & 0.128 [0.001,0.255] & 1.050 [0.843,1.288] \\
 & Oracle & 0.755 [0.726,0.780] & 0.192 [0.182,0.201] & 0.581 [0.546,0.628] & 0.035 [0.039,0.061] & 0.134 [0.018,0.254] & 0.836 [0.605,1.083] \\
\addlinespace[1pt]
\multirow{3}{*}{Qwen3.5-4B} & English & 0.684 [0.649,0.717] & 0.178 [0.168,0.188] & 0.535 [0.513,0.558] & 0.083 [0.076,0.098] & -1.444 [-2.045,-0.856] & 2.779 [2.201,3.402] \\
 & Pooled & 0.737 [0.708,0.765] & 0.155 [0.147,0.164] & 0.486 [0.463,0.512] & 0.042 [0.042,0.059] & 0.262 [0.014,0.459] & 1.064 [0.920,1.256] \\
 & Oracle & 0.756 [0.732,0.780] & 0.150 [0.141,0.159] & 0.465 [0.443,0.488] & 0.029 [0.032,0.047] & 0.016 [-0.201,0.229] & 1.037 [0.902,1.190] \\
\addlinespace[1pt]
\multirow{3}{*}{Qwen3.5-9B} & English & 0.690 [0.657,0.721] & 0.148 [0.137,0.161] & 0.465 [0.439,0.493] & 0.060 [0.051,0.072] & -5.292 [-6.596,-4.152] & 5.369 [4.495,6.378] \\
 & Pooled & 0.723 [0.693,0.752] & 0.133 [0.123,0.144] & 0.430 [0.402,0.459] & 0.036 [0.036,0.051] & 0.268 [-0.060,0.540] & 1.035 [0.879,1.243] \\
 & Oracle & 0.739 [0.711,0.765] & 0.129 [0.119,0.138] & 0.431 [0.402,0.463] & 0.029 [0.031,0.047] & 0.437 [0.088,0.725] & 0.821 [0.671,1.031] \\
\addlinespace[1pt]
\multirow{3}{*}{oss-low} & English & 0.681 [0.651,0.709] & 0.183 [0.171,0.196] & 0.632 [0.583,0.686] & 0.053 [0.050,0.077] & 0.406 [0.188,0.602] & 0.422 [0.318,0.568] \\
 & Pooled & 0.695 [0.664,0.725] & 0.178 [0.167,0.190] & 0.532 [0.508,0.559] & 0.033 [0.035,0.053] & -0.110 [-0.360,0.122] & 1.241 [1.037,1.462] \\
 & Oracle & 0.721 [0.694,0.746] & 0.172 [0.162,0.183] & 0.532 [0.504,0.561] & 0.029 [0.034,0.050] & 0.120 [-0.092,0.319] & 0.922 [0.778,1.102] \\
\addlinespace[1pt]
\multirow{3}{*}{oss-high} & English & 0.603 [0.553,0.647] & 0.125 [0.113,0.137] & 0.416 [0.387,0.445] & 0.078 [0.066,0.094] & 0.155 [-0.716,1.042] & 1.170 [0.574,1.803] \\
 & Pooled & 0.669 [0.630,0.706] & 0.116 [0.103,0.129] & 0.385 [0.353,0.418] & 0.030 [0.028,0.047] & 0.032 [-0.538,0.604] & 1.150 [0.847,1.494] \\
 & Oracle & 0.690 [0.646,0.728] & 0.112 [0.100,0.125] & 0.419 [0.372,0.472] & 0.033 [0.033,0.048] & 0.811 [0.302,1.111] & 0.647 [0.519,0.914] \\
\bottomrule
\end{tabular}%
}
\caption{Problem-clustered 95\% bootstrap intervals for selected-layer
self-probes. Each replicate computes a metric within each of the nine target
languages and then macro-averages, while resampling base problem IDs jointly
across translations. Each interval uses 2,000 replicates with seed 42.}
\label{tab:prediction-intervals-self}
\end{table*}

\begin{table*}[t]
\centering
\scriptsize
\setlength{\tabcolsep}{2.5pt}
\resizebox{\textwidth}{!}{%
\begin{tabular}{llrrrrrr}
\toprule
Model & Predictor & AUROC & Brier & NLL & ECE & Intercept & Slope \\
\midrule
\multirow{3}{*}{Qwen3-0.6B} & English raw & 0.769 [0.714,0.812] & 0.109 [0.100,0.120] & 0.465 [0.409,0.534] & 0.112 [0.109,0.124] & -1.192 [-1.462,-0.904] & 0.693 [0.486,0.966] \\
 & English + cal. & 0.769 [0.714,0.812] & 0.106 [0.094,0.118] & 0.385 [0.348,0.426] & 0.093 [0.084,0.104] & 0.906 [0.066,1.953] & 1.788 [1.254,2.494] \\
 & Pooled raw & 0.773 [0.725,0.814] & 0.088 [0.079,0.099] & 0.400 [0.346,0.463] & 0.035 [0.033,0.048] & -1.207 [-1.529,-0.736] & 0.311 [0.203,0.548] \\
\addlinespace[1pt]
\multirow{3}{*}{Qwen3-1.7B} & English raw & 0.759 [0.725,0.789] & 0.176 [0.167,0.185] & 0.547 [0.520,0.576] & 0.103 [0.099,0.118] & -0.287 [-0.469,-0.116] & 1.126 [0.883,1.390] \\
 & English + cal. & 0.759 [0.725,0.789] & 0.172 [0.162,0.182] & 0.539 [0.509,0.573] & 0.085 [0.085,0.103] & -0.087 [-0.290,0.107] & 0.963 [0.769,1.173] \\
 & Pooled raw & 0.777 [0.745,0.806] & 0.158 [0.149,0.168] & 0.520 [0.484,0.561] & 0.051 [0.047,0.071] & -0.192 [-0.395,0.084] & 0.821 [0.624,1.099] \\
\addlinespace[1pt]
\multirow{3}{*}{Qwen3-4B} & English raw & 0.729 [0.698,0.758] & 0.213 [0.205,0.220] & 0.624 [0.599,0.653] & 0.125 [0.115,0.146] & 0.301 [0.140,0.479] & 1.220 [0.927,1.554] \\
 & English + cal. & 0.729 [0.698,0.758] & 0.208 [0.199,0.216] & 0.614 [0.586,0.644] & 0.099 [0.097,0.115] & -0.033 [-0.147,0.084] & 0.939 [0.737,1.163] \\
 & Pooled raw & 0.741 [0.713,0.768] & 0.190 [0.183,0.198] & 0.573 [0.548,0.600] & 0.043 [0.046,0.063] & 0.050 [-0.092,0.192] & 0.924 [0.750,1.160] \\
\addlinespace[1pt]
\multirow{3}{*}{Qwen3-8B} & English raw & 0.723 [0.693,0.752] & 0.226 [0.218,0.233] & 0.648 [0.629,0.671] & 0.138 [0.121,0.162] & 0.700 [0.552,0.879] & 1.374 [1.142,1.673] \\
 & English + cal. & 0.723 [0.693,0.752] & 0.208 [0.198,0.217] & 0.609 [0.584,0.636] & 0.074 [0.072,0.089] & -0.015 [-0.142,0.109] & 0.994 [0.826,1.193] \\
 & Pooled raw & 0.733 [0.703,0.761] & 0.200 [0.191,0.209] & 0.606 [0.569,0.659] & 0.038 [0.042,0.063] & 0.212 [0.060,0.349] & 0.880 [0.606,1.230] \\
\addlinespace[1pt]
\multirow{3}{*}{Qwen3.5-4B} & English raw & 0.692 [0.659,0.723] & 0.193 [0.182,0.205] & 0.571 [0.546,0.599] & 0.133 [0.124,0.145] & -1.804 [-2.438,-1.144] & 2.490 [1.891,3.108] \\
 & English + cal. & 0.692 [0.659,0.723] & 0.190 [0.180,0.201] & 0.566 [0.543,0.592] & 0.141 [0.132,0.152] & -0.603 [-0.958,-0.222] & 1.693 [1.286,2.113] \\
 & Pooled raw & 0.727 [0.699,0.754] & 0.158 [0.150,0.168] & 0.492 [0.465,0.525] & 0.040 [0.040,0.056] & 0.300 [-0.011,0.550] & 0.975 [0.778,1.236] \\
\addlinespace[1pt]
\multirow{3}{*}{Qwen3.5-9B} & English raw & 0.668 [0.632,0.703] & 0.161 [0.146,0.177] & 0.503 [0.465,0.545] & 0.098 [0.084,0.117] & -3.840 [-4.996,-2.755] & 2.678 [2.142,3.252] \\
 & English + cal. & 0.668 [0.632,0.703] & 0.146 [0.135,0.158] & 0.455 [0.427,0.486] & 0.061 [0.058,0.075] & 0.094 [-0.231,0.413] & 1.007 [0.805,1.222] \\
 & Pooled raw & 0.715 [0.685,0.745] & 0.134 [0.124,0.145] & 0.426 [0.399,0.454] & 0.032 [0.032,0.046] & 0.234 [-0.114,0.519] & 1.030 [0.864,1.260] \\
\addlinespace[1pt]
\multirow{3}{*}{oss-low} & English raw & 0.584 [0.557,0.611] & 0.232 [0.212,0.253] & 2.110 [1.904,2.323] & 0.189 [0.172,0.211] & 0.030 [-3.729,0.451] & 0.144 [0.084,0.358] \\
 & English + cal. & 0.584 [0.557,0.611] & 0.196 [0.184,0.209] & 0.581 [0.555,0.609] & 0.061 [0.054,0.072] & -4.603 [-12.629,-2.334] & 5.652 [3.304,12.290] \\
 & Pooled raw & 0.712 [0.679,0.742] & 0.174 [0.164,0.185] & 0.522 [0.496,0.549] & 0.032 [0.035,0.054] & -0.006 [-0.225,0.206] & 1.141 [0.940,1.359] \\
\addlinespace[1pt]
\multirow{3}{*}{oss-high} & English raw & 0.545 [0.506,0.584] & 0.140 [0.123,0.158] & 1.350 [1.163,1.546] & 0.123 [0.111,0.138] & 1.330 [-0.402,3.074] & 0.051 [-0.061,0.179] \\
 & English + cal. & 0.545 [0.506,0.584] & 0.126 [0.112,0.141] & 0.419 [0.384,0.455] & 0.057 [0.049,0.068] & -2.562 [-17.614,9.624] & 2.491 [-4.027,10.514] \\
 & Pooled raw & 0.693 [0.649,0.734] & 0.114 [0.102,0.126] & 0.427 [0.378,0.486] & 0.048 [0.042,0.063] & 1.318 [0.923,1.554] & 0.300 [0.224,0.538] \\
\bottomrule
\end{tabular}%
}
\caption{Problem-clustered 95\% bootstrap intervals for the exact ETD
predictors. NLL uses aggregated rollout counts; calibration intercept and slope
are refit within each base-problem bootstrap replicate. Metrics macro-average
target-language-specific estimates, and all intervals use 2,000
replicates with seed 42.}
\label{tab:prediction-intervals-etd}
\end{table*}
