# Supplementary material for: Cross-lingual Calibration of Pre-Generation Success Probes for Multilingual LLM Routing
Source: arXiv:2610.06216 source file (2026-10-05)
Supplement: Supplementary file 7 [file appendix_routing_extensions.tex]

\begin{table}[t]
\centering
\scriptsize
\resizebox{\columnwidth}{!}{%
\begin{tabular}{llrrr}
\toprule
Extension & Val. choice & $\lambda$ & Success & Saving \\
\midrule
direct\_english & max (no match) & 0.00 & 83.2 & 18.0 \\
direct\_pooled & anchor match & 0.05 & 84.2 & 12.0 \\
ensemble\_english\_all & max (no match) & 0.00 & 80.5 & 22.6 \\
ensemble\_english\_local3 & max (no match) & 0.00 & 81.0 & 27.3 \\
ensemble\_english\_local7 & max (no match) & 0.00 & 81.1 & 29.2 \\
ensemble\_pooled\_all & anchor match & 0.10 & 84.3 & 22.4 \\
ensemble\_pooled\_local3 & anchor match & 0.10 & 84.5 & 22.5 \\
ensemble\_pooled\_local7 & anchor match & 0.10 & 84.4 & 22.8 \\
\bottomrule
\end{tabular}%
}
\caption{Appendix direct-probe and layer-ensemble routing. Direct routing charges
all candidate prefills; ensembles average fixed neighborhoods around the
validation-selected ETD layer or all layers.}
\label{tab:routing-extensions}
\end{table}
